# Supplementary material for: On Coherence in Bragg-Primakoff Axion Photoconversion
Source: arXiv:2309.01767 source file (2023-09-04)
Supplement: Supplementary file 1 [file appendix1.tex]

%%%%%%%%%%%%%%%%%%%%%%%%%%%%%%%%%%%%%%%%%%%%%%%%%%%
%
%  New template code for TAMU Theses and Dissertations starting Fall 2016.
%
%
%  Author: Sean Zachary Roberson 
%	 Version 3.16.09
%  Last updated 9/12/2016
%
%%%%%%%%%%%%%%%%%%%%%%%%%%%%%%%%%%%%%%%%%%%%%%%%%%%

%%%%%%%%%%%%%%%%%%%%%%%%%%%%%%%%%%%%%%%%%%%%%%%%%%%%%%%%%%%%%%%%%%%%%%
%%                           APPENDIX A 
%%%%%%%%%%%%%%%%%%%%%%%%%%%%%%%%%%%%%%%%%%%%%%%%%%%%%%%%%%%%%%%%%%%%%

\phantomsection

\chapter{\uppercase{Statistics and Probability Theory}}
\label{app:stats}

Suppose we have a set of independent background expectations $B_i$ and an expected signal $S_i$ across bins $i=1,\dots,\nu$. In the absence of data, we can ask the question: ``If our experiment sees data consistent with background-only, does the median value of the $\chi^2$ distribution tested against our $S+B$ model exceed the $1-\alpha$ quantile of the background-only $\chi^2$ distribution?"

To do this we generate a set of independent, normally distributed fake data $d_i \sim N(B_i, \sqrt{B_i})$. In the limit of a large number of pseudo-experiments, the $1-\alpha$ quantile of this distribution approaches the theoretical limit $F^{-1}(1-\alpha, \nu)$. Now consider the expectation value of the $\chi^2$ tested against our $S+B$ expectation;

\begin{align}
    \EX[\chi^2_{S+B}] &= \EX\bigg[\sum_{i=1}^\nu \dfrac{(d_i - S_i - B_i)^2}{B_i} \bigg] \nonumber \\
    &= \sum_{i=1}^\nu \bigg( \EX\bigg[ \dfrac{d_i - S_i - B_i}{\sqrt{B_i}} \bigg]  \bigg)^2 + \Var\bigg[  \dfrac{d_i - S_i - B_i}{\sqrt{B_i}}\bigg] \nonumber \\
    &= \sum_{i=1}^\nu \bigg( \EX\bigg[ \dfrac{d_i}{\sqrt{B_i}}\bigg] -  \EX\bigg[ \dfrac{S_i + B_i}{\sqrt{B_i}} \bigg]  \bigg)^2 + \frac{1}{B_i}\Var[d_i] \nonumber \\
    &= \sum_{i=1}^\nu \bigg( \dfrac{B_i}{\sqrt{B_i}} -  \dfrac{S_i + B_i}{\sqrt{B_i}} \bigg)^2 + \frac{1}{B_i}B_i \nonumber \\
    &= \sum_{i=1}^\nu \bigg( \dfrac{S_i^2}{B_i} + 1 \bigg)  \nonumber \\
    &=  \nu + \sum_{i=1}^\nu\dfrac{S_i^2}{B_i}
\end{align}

Above we used the linearity of expectation values and the assumption that $d_i$ are independent, and that $\Var[d_i] = (\sqrt{B_i})^2$. The test statistic that I used is the second term;
\begin{equation}
    t \equiv \sum_{i=1}^\nu\dfrac{S_i^2}{B_i} = \EX[\chi^2_{S+B}] - \nu
\label{eq:tstat}
\end{equation}
We can then make use of the following approximation of the median of a $\chi^2$ distribution with $k$ degrees of freedom
\begin{equation}
    \textrm{Median}[\chi^2] \simeq k \bigg(1 - \frac{2}{9 k} \bigg)^3 = k - \frac{2}{3} + \mathcal{O}(k^{-1})
\end{equation}
Since $\EX[\chi^2_k] = k$, for $k \gtrsim 13$ we have $\textrm{Median}[\chi^2] \simeq \EX[\chi^2_k]$ to within 5\% error. Our original question requires that
\begin{equation}
     \textrm{Median}[\chi_{S+B}^2] > F^{-1} (1-\alpha, \nu) \equiv \chi^2_\alpha
\end{equation}
it follows that we need to find the smallest signal such that
\begin{equation}
     t \gtrsim \chi^2_\alpha - \nu .
     \label{eq:ineq}
\end{equation}
For example, if we take $\nu = 24$ bins, and $\alpha = 0.1$, then we have
\begin{equation}
    t \gtrsim 33.2 - 24 \simeq 9.2
\end{equation}
This differs from the critical value I chose, $t=4.61$ based on 2 free parameters. It seems, then, that Eq.~\ref{eq:ineq} \textit{could} be used for CL setting in lieu of running pseudo-experiments only under the following special conditions;
\begin{enumerate}
    \item If the data $d_i$ can be safely assumed to be independent
    \item If the data $d_i$ can be safely assumed to be normally distributed
    \item If the number of bins $\nu \gtrsim \mathcal{O}(10)$, otherwise the approximation for $\textrm{Median}[\chi^2]$ loses precision
\end{enumerate}

\clearpage

\begin{figure}
    \centering
    \includegraphics[width=0.5\textwidth]{graphic/bkg_pseudo_experiments.png}
    \caption{Pseudo-experiment data for a given background over $\nu = 30$ bins, and a comparison of the empirically calculated and theoretical positions of the median $\chi^2$ and $\chi^2_{90\%}$ values with 10,000 psuedo-experiments. The empirical median and theoretical lines lie on top of each other.}
    \label{fig:my_label}
\end{figure}

\begin{figure}
    \centering
    \includegraphics[width=0.5\textwidth]{graphic/bkg_vs_signal_chi2.png}
    \caption{Comparison between the background $\chi^2$ and the signal-plus-background $\chi^2$ distributions, their medians and p-value locations, and the distance $t$ given in Eq.~\ref{eq:tstat} for $\nu = 30$ bins. The $\chi^2_{B,0.9}$ and $\textrm{Med}[S+B]$ lines lie on top of each other. It is interesting that the requirement $\mathrm{Median}[\chi^2_{S+B}] \to \chi^2_{B,0.9}$ is not the same as asking that $\mathrm{Median}[\chi^2_B] \to \chi^2_{S,0.1}$; the latter would require a slightly more conservative distance measure between the two distributions. I think this is because the $\chi^2$ distribution still has a noticeable asymmetry for $\nu = 30$ degrees of freedom; this discrepancy should vanish in the limit of large $\nu$.}
    \label{fig:my_label}
\end{figure}
