# Supplementary material for: On Coherence in Bragg-Primakoff Axion Photoconversion
Source: arXiv:2309.01767 source file (2023-09-04)
Supplement: Supplementary file 2 [file appendix2.tex]

%%%%%%%%%%%%%%%%%%%%%%%%%%%%%%%%%%%%%%%%%%%%%%%%%%%
%
%  New template code for TAMU Theses and Dissertations starting Fall 2016.
%
%
%  Author: Sean Zachary Roberson 
%	 Version 3.16.09 
%  Last updated 9/12/2016
%
%%%%%%%%%%%%%%%%%%%%%%%%%%%%%%%%%%%%%%%%%%%%%%%%%%%

%%%%%%%%%%%%%%%%%%%%%%%%%%%%%%%%%%%%%%%%%%%%%%%%%%%%%%%%%%%%%%%%%%%%%%
%%                           APPENDIX B
%%%%%%%%%%%%%%%%%%%%%%%%%%%%%%%%%%%%%%%%%%%%%%%%%%%%%%%%%%%%%%%%%%%%%

\phantomsection

\chapter{\uppercase {Monte Carlo Methods}}
\label{app:mc}

\section{$2\to2$ Scattering}
\label{app:2to2}
For any $2\to 2$ process $\phi_1 (p_1) \phi_2 (p_2) \rightarrow \phi_3 (p_3) \phi_4 (p_4)$, we can express the Lorentz invariant amplitude as a function of Mandelstam $s, t$ as $\mathcal{A}(s,t) = \braket{\mid\mathcal{M}(s,t)\mid^2}$, for Mandelstam definitions
\begin{align}
    s &= (p_1 + p_2)^2 = (p_3 + p_4)^2 \\
    t &= (p_1 - p_3)^2 = (p_2 - p_4)^2 \\
    u &= (p_1 - p_4)^2 = (p_2 - p_3)^2 \\
    u &= m_1^2 + m_2^2 + m_3^2 + m_4^2 - s - t
\end{align}
Given masses $m_i$, $i=1,\dots,4$ and incoming 4-momenta $p_1^\mu$ and $p_2^\mu$, we can simulate the outgoing 4-momenta $p_3^\mu$ and $p_4^\mu$ as follows;

\begin{enumerate}
    \item Find the Lorentz boost velocity $v$ to transform $p_1^\mu$ and $p_2^\mu$ to the CM frame. In the special case of a fixed target with an incident beam along the $z$-direction, e.g. $p_1^\mu = (E_1, 0, 0, p_1)$ and $p_2^\mu = (m_2, 0, 0, 0)$, we have
        \begin{align}
            v &= \dfrac{p_1}{m_2 + E_1} \\
            \to \gamma &= (1 - v^2)^{-1/2}
        \end{align}
    \item In the CM frame, the energies of the outgoing particles are fixed, so $t$ is purely a function of $\cos\theta$;
        \begin{equation}
            t(\cos\theta^*) = m_1^2 + m_3^2 - 2E^*_1 E^*_3 + 2 p^*_1 p^*_3 \cos\theta^*
        \end{equation}
    where
        \begin{equation}
            \mid {p_{1,3}^*}\mid^2 = \dfrac{(s - m_{1,3}^2 - m_{2,4}^2)^2 - 4m_{1,3}^2 m_{2,4}^2}{4s}
        \end{equation}
        \begin{equation}
            E^*_{1,3} = \sqrt{\mid p_{1,3}^* \mid^2 - m_{1,3}^2}
        \end{equation}
    \item Draw $j=1,\dots,N$ random variates $u_j \sim U(-1,1)$ and find $t_j(u_j)$
    \item The differential scattering cross section in the CM frame is given by 
    \begin{equation}
        \dfrac{d\sigma}{dt} = \dfrac{1}{16\pi(s-(m_1 + m_2)^2)(s-(m_1 - m_2)^2)} \mid \mathcal{M}(s,t_j) \mid^2
    \end{equation}
    with
    \begin{equation}
        \dfrac{d\sigma}{d(\cos\theta^*)} = 2 p^*_1 p^*_3 \dfrac{d\sigma}{dt}
    \end{equation}
    Therefore, the MC weights in the center of momentum frame, $w_j^\textrm{CM}$, are given by
    \begin{equation}
        w_j^\textrm{CM} = \dfrac{2}{N} 2 p^*_1 p^*_3 \dfrac{d\sigma(s, t_j)}{dt}
    \end{equation}
    where the factor of $2/N$ is the MC volume factor.
    
    \item Boost to the lab frame, transforming the outgoing 4-momenta as
    \begin{align}
        E_3 &= \gamma (E_3^* + \beta p_3^* \cos\theta^*) \\
        p_3 \cos\theta &= \gamma (p_3^* \cos\theta^* + \beta E_3^*)
    \end{align}
    which implies
    \begin{align}
        \dfrac{d\sigma}{dE_3} &= \bigg( \dfrac{1}{\gamma \beta p_3^*}\bigg)\dfrac{d\sigma}{d(\cos\theta^*)} \nonumber \\
        &= \dfrac{2 p_1^*}{\gamma \beta} \dfrac{d\sigma}{dt}.
    \end{align}
    However, we need to multiply by the MC volume $E_3^{max} - E_3^{min} = 2\gamma \beta p_3^*$, leaving the differential energy weights simply as
    \begin{align}
        w_j^\textrm{energy} &= \frac{1}{N} 2\gamma\beta p_3^* \dfrac{d\sigma}{dE_3} \nonumber \\
        &= w_j^\textrm{CM}
    \end{align}
    More generally, the weights pickup a Jacobian factor $J_j$, depending on what variable we want to transform to (\cite{Catchen_78});
    \begin{align}
        J\bigg[\dfrac{p_3^*, \Omega^*}{p_3, \Omega}\bigg] &= \dfrac{p_3^2 E_3^*}{p_3^{*2} E_3} \\
        J\bigg[\dfrac{\Omega^*}{\Omega}\bigg] &= \bigg(\dfrac{v}{v^*}\bigg)^2 (\cos\theta \cos\theta^* + \sin\theta \sin\theta^* \cos(\phi - \phi^*)) \nonumber \\
        &= \bigg(\dfrac{v}{v^*}\bigg)^2 \cos\delta
    \end{align}
    Where $\delta$ is the angle between $\vec{v}$ and $\vec{v}^*$. The angles can be related through the Lorentz transformation for a simple boost along the $z$-axis;
    \begin{align}
        \theta &= \arccos \bigg\{\dfrac{\gamma (p_3^* \cos\theta^* + \beta E_3^*)}{\sqrt{(\gamma (E_3^* + \beta p_3^* \cos\theta^*))^2 - m_3^2)}}\bigg\} \\
        \phi &= \phi^*
    \end{align}
    Therefore, we have enough to write the differential cosine distribution in the lab frame;
    \begin{equation}
        \dfrac{d\sigma}{d(\cos\theta)} = \bigg(\dfrac{v}{v^*}\bigg)^2 \cos\delta \dfrac{d\sigma}{d(\cos\theta^*)}
    \end{equation}
    and the differential cosine weights are
    \begin{equation}
        w_j^\textrm{cosine} = \frac{2}{N}\bigg(\dfrac{v}{v^*}\bigg)^2 \cos\delta \dfrac{d\sigma}{d(\cos\theta^*)} = \bigg(\dfrac{v}{v^*}\bigg)^2 \cos\delta \, \, w_j^\textrm{CM}
    \end{equation}
\end{enumerate}
At the end of the simulation, for $N$ samples one should have
\begin{equation}
u_j \sim U(-1, 1) \, \, \to 
    E_{3,j}, \cos\theta_j, w_j^\textrm{cosine}, w_j^\textrm{energy}
\end{equation}

\section{3 Body Decays}
\label{app:3body}

For the charged meson 3-body decay $M(P) \to \ell(p_1) \nu(p_2) a(p_3)$, we make use of the Dalitz variables $m_{ij}^2 = (p_i + p_j)^2$. In the lab frame, we have
\begin{align}
    m_{12}^2 &= (p_1 + p_2)^2 = (P - p_3)^2 = M^2 - 2ME_a + m_a^2 \\
    m_{23}^2 &= (p_2 + p_3)^2 = (P - p_1)^2 = M^2 - 2ME_\ell + m_\ell^2 \\
    m_{13}^2 &= (p_1 + p_3)^2 = (P - p_2)^2 = M^2 - 2ME_\nu \\
    m_{13}^2 &= M^2 + m_\ell^2 + m_a^2 - m_{12}^2 - m_{23}^2 .
\end{align}
This set of variables allows us to write
\begin{equation}
    d\Gamma = \dfrac{1}{(2\pi)^3 32 M^3} \braket{|M|^2} dm_{23}^2 dm_{12}^2
\end{equation}
and re-express $m_{12}^2$ in terms of $E_a$, since $|dm_{12}^2| = 2MdE_a$, allowing us to integrate over $m_{23}^2$;
\begin{equation}
    \dfrac{d\Gamma}{dE_a} =  \int^{(m_{23}^2)_{max}}_{(m_{23}^2)_{min}} \dfrac{1}{(2\pi)^3 16 M^2} \braket{|M|^2} dm_{23}^2 .
\end{equation}
This has bounds
\begin{equation}
    (m_{23}^2)^{max}_{min} = (E_2^* + E_3^*)^2 - \bigg(E_2^* \mp \sqrt{{E_3^*}^2 - m_a^2}\, \bigg)
\end{equation}
with the starred energies defined as
\begin{align}
    E_2^* &= \dfrac{m_{12}^2 - m_\ell^2}{2 m_{12}} \\
    E_3^* &= \dfrac{M^2 - m_{12}^2 - m_a^2}{2 m_{12}}
\end{align}
Finally, we can integrate over $E_a$ making use of the fact that $m_\ell^2 < m_{12}^2 < M^2 + m_a^2 - 2Mm_a$ to get the $E_a$ limits;
\begin{equation}
    m_a < E_a < \dfrac{M^2 + m_a^2 - m_\ell^2}{2 M}.
\end{equation}

\section{Log-space Monte Carlo Integration}

In MC integration, the objective may be to find the integral of $f(x)$ over the interval $(x_1, x_2)$;
\begin{equation}
    I = \int_{x_1}^{x_2} f(x) dx
\end{equation}
Traditional MC gives the prescription
\begin{equation}
    I = \lim_{N\to\infty} \dfrac{(x_2 - x_1)}{N} \sum_{i=1}^N f(X_i).
\end{equation}
for $N$ samples $X_i \in \{X_1,\cdots,X_N\}$ randomly generated over the interval. If we instead move to log-space, with $d \ln x = \frac{1}{x} dx$,
\begin{equation}
    I = \int_{\ln x_1}^{\ln x_2} x f(x) d \ln x
\end{equation}
A quick matching of formulae leads to the analogous MC formula when integrating over log-space:
\begin{equation}
    I \approx \dfrac{\ln x_2 - \ln x_1}{N} \sum_{i=1}^N f(X_i) \cdot X_i = \dfrac{\ln \frac{x_2}{x_1}}{N} \sum_{i=1}^N f(X_i) \cdot X_i.
\end{equation}
Note that now, we randomly sample over $\ln x$ as $X_i \sim e^{U(\ln x_1, \ln x_2)}$. In python, for example, this might look like
\begin{align}
    &\texttt{import numpy as np} \nonumber \\
    &\texttt{from numpy import exp, log} \nonumber \\
    &\texttt{x\_1, x\_2, n\_samples = 1.0e-7, 10.0, 10000} \nonumber \\
    &\texttt{x = exp(np.random.uniform(log(x\_1), log(x\_2), n\_samples))} \nonumber
\end{align}
In $d$-dimensions, this generalizes to
\begin{equation}
    I \approx \dfrac{V_d}{N} \sum_{i=1}^N f(\vec{R}_i) \cdot \prod_{j=1}^d X_{i,j}.
\end{equation}
where the samples are now random vectors $\vec{R}_i = (X_{i,1}, \cdots, X_{i,d})$ and the log-volume is taken over the closed surface $\Omega$; $V_d = \int_\Omega d\ln \vec{r}$.

In 2 dimensions, for example, integrating over a rectangular domain $\{(x_1, x_2), (y_1, y_2)\}$, we would generate $N$ sample pairs $\vec{R}_i = (X_i, Y_i)$ and get
\begin{equation}
    \int_{y_1}^{y_2} \int_{x_1}^{x_2} f(x,y) dx dy \approx \dfrac{\ln\frac{x_2}{x_1} \ln\frac{y_2}{y_1}}{N} \sum_{i=1}^N X_i Y_i f(X_i,Y_i)
\end{equation}
If we instead use base-10, we can use the fact that $d \log_{10} x = \frac{1}{\ln (10) x} dx$. In that case, we take $V_d^{10} = \int_{\Omega} d\log_{10}\vec{r}$ and
\begin{equation}
    I \approx \dfrac{V^{10}_d}{N} \sum_{i=1}^N f(\vec{R}_i) \cdot (\ln(10))^d \cdot \prod_{j=1}^d X_{i,j},
\end{equation}
giving
\begin{equation}
    \int_{y_1}^{y_2} \int_{x_1}^{x_2} f(x,y) dx dy \approx \dfrac{\log_{10}\frac{x_2}{x_1} \log_{10}\frac{y_2}{y_1}}{N} (\ln(10))^2 \sum_{i=1}^N X_i Y_i f(X_i,Y_i)
\end{equation}
\clearpage
