# Supplementary material for: On Coherence in Bragg-Primakoff Axion Photoconversion
Source: arXiv:2309.01767 source file (2023-09-04)
Supplement: Supplementary file 3 [file appendix3.tex]

%%%%%%%%%%%%%%%%%%%%%%%%%%%%%%%%%%%%%%%%%%%%%%%%%%%
%
%  New template code for TAMU Theses and Dissertations starting Fall 2016.
%
%
%  Author: Sean Zachary Roberson 
%	 Version 3.16.09 
%  Last updated 9/12/2016
%
%%%%%%%%%%%%%%%%%%%%%%%%%%%%%%%%%%%%%%%%%%%%%%%%%%%

%%%%%%%%%%%%%%%%%%%%%%%%%%%%%%%%%%%%%%%%%%%%%%%%%%%%%%%%%%%%%%%%%%%%%%
%%                           APPENDIX C
%%%%%%%%%%%%%%%%%%%%%%%%%%%%%%%%%%%%%%%%%%%%%%%%%%%%%%%%%%%%%%%%%%%%%

\phantomsection

\chapter{\uppercase {Matrix Elements}}
\label{app:mc}

\section{Axioelectric Effect}

\section{Compton Scattering}
The Compton scattering channel depicted in Fig.~\ref{fig:compton}, left (and inverse Compton scattering, right) is analogous to the SM process of the same name, where the SM photon is replaced with the ALP $(a)$. Depending on the ALP mass and energy, the kinematics and momentum fraction shared by the outgoing final states in both the forward and inverse processes can change, which I will illustrate below.
\begin{figure}
    \centering
    \begin{tikzpicture}
        \begin{feynman}
         
        \vertex (i1) {\(e^-\)};
         \vertex [right=1.4cm of i1] (v1);
         \vertex [above left=1.0cm of v1] (i2) {\(\gamma\)};
        \vertex [right=1.0cm of v1] (v2);
        \vertex [above right=1.0cm of v2] (o1) {\(a\)};
        \vertex [right=1.0cm of v2] (o2) {\(e^-\)};

         \diagram* {
           (i1) -- [fermion] (v1) -- [fermion] (v2) -- [fermion] (o2),
           (i2) -- [boson] (v1),
           (v2) -- [scalar] (o1),
         };
        \end{feynman}
    \end{tikzpicture}
    \begin{tikzpicture}
        \begin{feynman}
        \vertex (o1);
         \vertex [right=1.4cm of o1] (f1) {\(a\)};
         \vertex [left=1.4cm of o1] (i1){\(e^-\)} ;
         \vertex [below=1.4cm of o1] (o2);
         \vertex [right=1.4cm of o2] (f2) {\(e^-\)};
         \vertex [left=1.4cm of o2] (i2) {\(\gamma\)};

         \diagram* {
           (i1) -- [fermion] (o1) -- [scalar] (f1),
           (o1) -- [fermion] (o2),
           (i2) -- [boson] (o2),
           (o2) -- [ fermion] (f2),
         };
        \end{feynman}
    \end{tikzpicture}\\
    \begin{tikzpicture}
        \begin{feynman}
        \vertex (i1) {\(e^-\)};
         \vertex [right=1.4cm of i1] (v1);
         \vertex [above left=1.0cm of v1] (i2) {\(a\)};
        \vertex [right=1.0cm of v1] (v2);
        \vertex [above right=1.0cm of v2] (o1) {\(\gamma\)};
        \vertex [right=1.0cm of v2] (o2) {\(e^-\)};

         \diagram* {
           (i1) -- [fermion] (v1) -- [fermion] (v2) -- [fermion] (o2),
           (i2) -- [scalar] (v1),
           (v2) -- [boson] (o1),
         };
        \end{feynman}
    \end{tikzpicture}
    \begin{tikzpicture}
        \begin{feynman}
         \vertex (o1);
         \vertex [right=1.4cm of o1] (f1) {\(e^-\)};
         \vertex [left=1.4cm of o1] (i1){\(a\)} ;
         \vertex [below=1.4cm of o1] (o2);
         \vertex [right=1.4cm of o2] (f2) {\(\gamma\)};
         \vertex [left=1.4cm of o2] (i2) {\(e^-\)};

         \diagram* {
           (i1) -- [scalar] (o1) -- [fermion] (f1),
           (o1) -- [anti fermion] (o2),
           (i2) -- [fermion] (o2),
           (o2) -- [ boson] (f2),
         };
        \end{feynman}
    \end{tikzpicture}
    \caption{Compton and inverse-Compton scattering for ALP production and detection.}
    \label{fig:compton}
\end{figure}

One may refer to \cite{Brodsky:1986mi}, where the differential cross section was worked out. To fill in some details, the spin-averaged matrix element is given as
\begin{align}
\frac{1}{4}|\mathcal{M}|^2 &= g_{ea}^2e^2\bigg[ \frac{m^4 + m^2 (3m_a^2 - 2s - t) + s(s+t-m_a^2)}{(u-m^2)^2}  \nonumber \\
& + \frac{m^4 + m^2 (3m_a^2 - 2s - t) + s(s+t-m_a^2)}{(s-m^2)^2} \nonumber \\
&+ 2\frac{m^4 + m^2 (3m_a^2 - 2s - t) - (m_a^2 - s)(s+t)}{(s-m^2)(u-m^2)}\bigg]
\end{align}

It has a differential scattering cross-section, in light-cone coordinates,
\begin{equation}
    \frac{d\sigma_C}{dx} = \frac{Z \pi g_{aee}^2 \alpha x}{4\pi(s- m_e^2)(1-x)}\bigg[x - \frac{2m_a^2 }{(s-m_e^2)^2} \bigg(s - \frac{m_e^2}{1-x} -\frac{m_a^2}{x}\bigg)\bigg]
\end{equation}
One may perform a change of variables to the lab frame using $s-m_e^2 = 2E_\gamma m_e$ and $x = 1 - \frac{E_a}{E_\gamma} + \frac{m_a^2}{2 E_\gamma m_e}$. In the limit that $s>>m_a$, integrating gives
\begin{equation}
    \sigma_C = \dfrac{\pi \alpha g_{aee}^2}{4\pi s} \bigg(\dfrac{10 m_e^2 - 3 s}{2 s} + \ln \dfrac{m_e^2 + s}{m_e^2} \bigg)
\end{equation}
In one is interested in the cross-section at any part of the phase space, it is given in ~\cite{Gondolo:2008dd}:
\begin{equation}
    \sigma = \dfrac{\alpha g_{aee}^2 p}{8s\cdot k} \bigg[ -3 + \dfrac{m_e^2 - m_a^2}{s} + \dfrac{8 m_a^2 s}{(s-m_e^2)^2} + \bigg( 1 - \dfrac{2 m_a^2}{s - m_e^2} + \dfrac{2m_a^2 (m_a^2 - 2 m_e^2)}{(s-m_e^2)^2} \bigg)\dfrac{\sqrt{s}}{p} \ln \dfrac{2p_0 k_0 + 2pk - m_a^2}{2 p_0 k_0 - 2pk - m_a^2} \bigg]
\end{equation}
where
\begin{align}
    p_0 = \dfrac{s-m_e^2 + m_a^2}{2\sqrt{s}} \\
    p = \sqrt{p_0^2 - m_a^2} \\
    k_0 = \dfrac{s + m_e^2}{2\sqrt{s}} \\
    k = \sqrt{s} - k_0 \\
\end{align}

The inverse Compton scattering process, ($a + e^- \to \gamma + e^-$, for ALP detection (Fig.~\ref{fig:compton}, right) can be found in~\cite{Avignone:1988bv} as well. This process produces visible energy in the final state electron recoil and outgoing photon. The total cross section is~\cite{Avignone:1988bv,Gondolo:2008dd};
\begin{equation}
    \sigma(E_a) = \dfrac{g_{ae}^2 \alpha}{8 m_e p_a} \bigg[ \frac{2 m_e^2 (E_a + m_e) y}{(y + m_e^2)^2} + \frac{4 m_e (m_a^4 + 2m_e^2 m_a^2 - 4m_e^2 E_a^2)}{y (y + m_e^2)} + \frac{4 m_e^2 p_a^2 + m_a^4}{p_a y} \ln \bigg(\frac{m_e + E_a + p_a}{m_e + E_a - p_a} \bigg) \bigg]
\end{equation}
where $y = m_a^2 + 2 m_e E_a$.

\clearpage
